# Supplementary material for: Double Machine Learning and Automated Confounder Selection -- A Cautionary Tale
Source: arXiv:2108.11294 ancillary file (2023-05-24)
Supplement: Supplementary file 1 [file Huenermund_etal_Online_Supplement.pdf]

# DML and Automated Confounder Selection: Online Supplement

PAUL HÜNERMUND<sup>†</sup>      BEYERS LOUW<sup>‡</sup>      ITAMAR CASPI<sup>\*</sup>

<sup>†</sup> *Copenhagen Business School, Kilevej 14A, Frederiksberg, 2000, DK.*

E-mail: [phu.si@cbs.dk](mailto:phu.si@cbs.dk)

<sup>‡</sup> *Maastricht University, Tongersestraat 53, 6211 LM Maastricht, NL.*

E-mail: [jb.louw@maastrichtuniversity.nl](mailto:jb.louw@maastrichtuniversity.nl)

<sup>\*</sup> *Bank of Israel, P.O.Box 780, 91007, Jerusalem, IL*

E-mail: [itamar.caspi@boi.org.il](mailto:itamar.caspi@boi.org.il)

This version: February 8, 2022

First version: August 26, 2021

## Summary

Online supplement to Hünernmund, Louw, and Caspi (2022), which contains additional figures and simulation results that were not included in the main text due to space limitations.

**Keywords:** *Double/Debiased Machine Learning, Directed Acyclic Graphs, Structural Causal Models, Backdoor Adjustment, Collider Bias*

## 1. SIMULATION PARAMETERIZATION

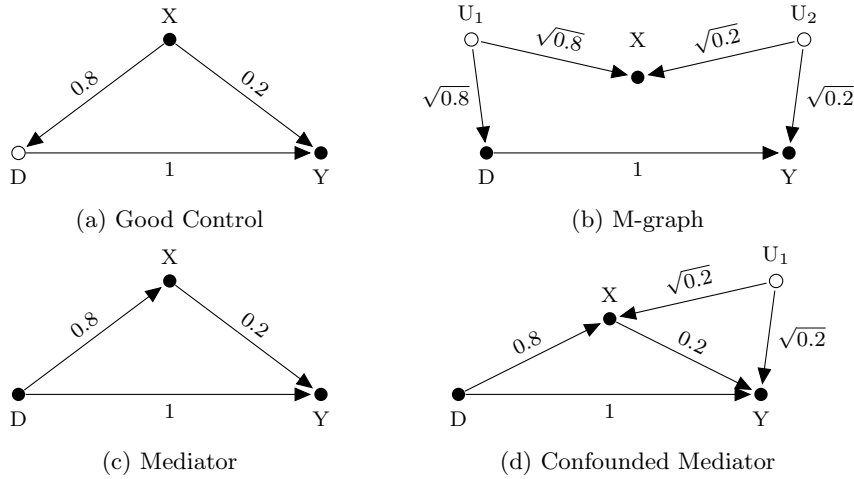

**Figure 1:** Parameterization used to produce results in Figure 1 in the main text.

2. DML PERFORMANCE WITH  $L_2$ -BOOSTING**Table 1:** Bias obtained from DML with  $l_2$ -Boosting ( $\theta_0 = 1$ )

| $(b_1, b_2) =$      | (0.8, 0.2) | (0.6, 0.4) | (0.5, 0.5) | (0.4, 0.6) | (0.2, 0.8) |
|---------------------|------------|------------|------------|------------|------------|
| Good Control        | -0.038     | -0.023     | -0.016     | -0.010     | -0.003     |
| M-graph             | -0.219     | -0.266     | -0.273     | -0.269     | -0.224     |
| Mediator            | -0.149     | -0.115     | -0.086     | -0.049     | -0.009     |
| Confounded Mediator | -0.592     | -0.533     | -0.470     | -0.397     | -0.234     |
| $q =$               | 1          | 5          | 10         | 20         | 50         |
| Good Control        | -0.110     | -0.095     | -0.037     | 0.091      | 0.211      |
| M-graph             | -0.156     | -0.210     | -0.218     | -0.216     | -0.201     |
| Mediator            | -0.129     | -0.141     | -0.143     | -0.115     | 0.196      |
| Confounded Mediator | -0.249     | -0.478     | -0.594     | -0.674     | -0.781     |

(a) Good Control

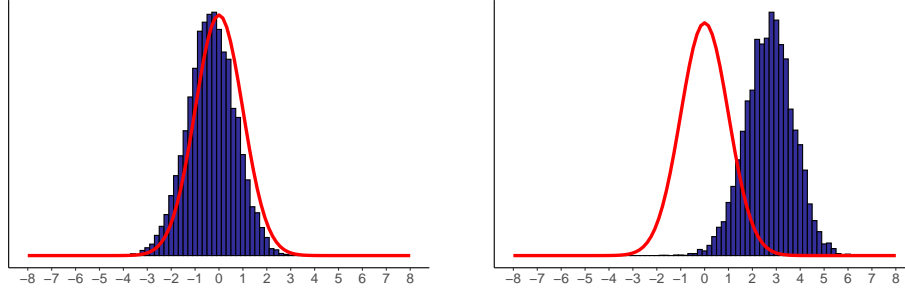

(b) M-graph

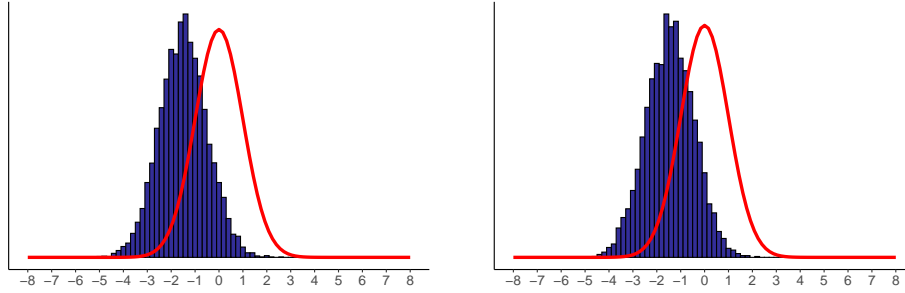

(c) Mediator (direct effect)

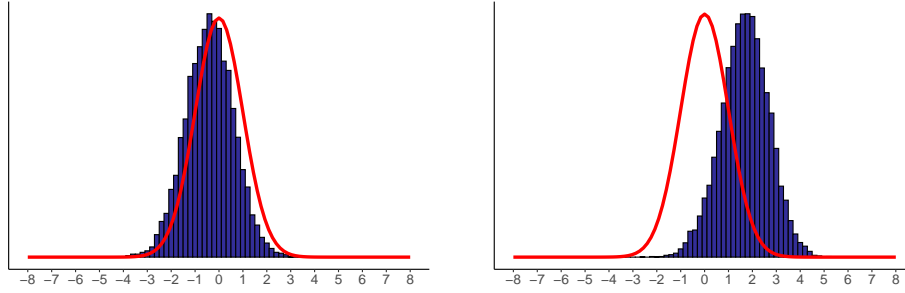

(d) Confounded Mediator (direct effect)

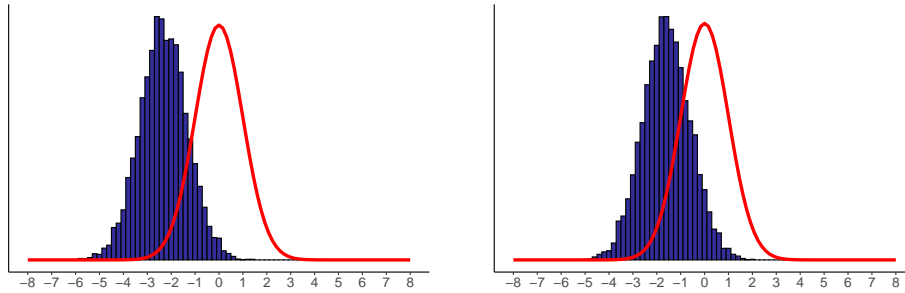

**Figure 2:** DML Performance in the presence of bad controls using  $l_2$ -boosting

3. SIMULATION RESULTS WITH VARYING  $P$  AND  $N$ **Table 2:** Bias obtained from DML with  $p = 100$  and  $n = 1,000$  ( $\theta_0 = 1$ )

| $(b_1, b_2) =$      | (0.8, 0.2) | (0.6, 0.4) | (0.5, 0.5) | (0.4, 0.6) | (0.2, 0.8) |
|---------------------|------------|------------|------------|------------|------------|
| Good Control        | 0.000      | 0.000      | 0.000      | 0.000      | 0.000      |
| M-graph             | -0.119     | -0.172     | -0.179     | -0.174     | -0.126     |
| Mediator            | 0.000      | 0.000      | -0.001     | -0.001     | -0.001     |
| Confounded Mediator | -0.534     | -0.480     | -0.417     | -0.343     | -0.177     |
| $q =$               | 1          | 5          | 10         | 20         | 50         |
| Good Control        | 0.000      | 0.000      | 0.000      | 0.000      | 0.000      |
| M-graph             | -0.054     | -0.105     | -0.120     | -0.128     | -0.135     |
| Mediator            | 0.000      | -0.001     | -0.001     | -0.001     | -0.005     |
| Confounded Mediator | -0.134     | -0.401     | -0.534     | -0.642     | -0.725     |

**Table 3:** Bias obtained from DML with  $p = 500$  and  $n = 500$  ( $\theta_0 = 1$ )

| $(b_1, b_2) =$      | (0.8, 0.2) | (0.6, 0.4) | (0.5, 0.5) | (0.4, 0.6) | (0.2, 0.8) |
|---------------------|------------|------------|------------|------------|------------|
| Good Control        | -0.001     | -0.001     | -0.001     | -0.001     | -0.001     |
| M-graph             | -0.120     | -0.063     | -0.179     | -0.175     | -0.128     |
| Mediator            | -0.002     | -0.001     | -0.001     | -0.001     | -0.001     |
| Confounded Mediator | -0.533     | -0.479     | -0.416     | -0.342     | -0.177     |
| $q =$               | 1          | 5          | 10         | 20         | 50         |
| Good Control        | -0.001     | -0.001     | -0.001     | -0.002     | -0.005     |
| M-graph             | -0.054     | -0.105     | -0.120     | -0.129     | -0.136     |
| Mediator            | -0.003     | -0.003     | -0.003     | -0.003     | -0.001     |
| Confounded Mediator | -0.132     | -0.398     | -0.533     | -0.638     | -0.726     |

## 4. GENDER WAGE GAP APPLICATION: ADDITIONAL RESULTS

**Table 4:** Effect of gender on log wages using PSID, incl. *marital status* but without interactions.

| Wave =                          | 1981    | 1990    | 1999    | 2007    | 2009    | 2011    |
|---------------------------------|---------|---------|---------|---------|---------|---------|
| DML incl. <i>marital status</i> | -0.285  | -0.156  | -0.181  | -0.199  | -0.197  | -0.177  |
| w/o interactions                | (0.021) | (0.019) | (0.020) | (0.019) | (0.019) | (0.020) |

## 5. R CODE USED FOR PRODUCING SIMULATION RESULTS

```

1  library(hdm)
2
3  set.seed(12345)
4
5  s <- 10000 # number of simulations
6  n <- 100   # sample size
7  p <- 100   # number of parameters
8  q <- 10     # number of variables with non-zero coefficients
9  theta <- 1  # (direct) effect of d
10 b1 <- 0.8   # Cov(d,x)
11 b2 <- 0.2   # Cov(y,x|d)
12
13 res <- data.frame(matrix(NA, nrow=s, ncol=8))
14 colnames(res) <- c("dml1", "post.lasso1", "dml2", "post.lasso2",
15                  "dml3", "post.lasso3", "dml4", "post.lasso4")
16
17 #####
18 ### 1. Good Control
19 #####
20 for (i in 1:s){
21   X <- matrix(rnorm(n * p), ncol = p)
22   colnames(X) <- paste("X", 1:p, sep = " ")
23
24   beta <- c(rep(b2, q), rep(0, p - q))
25   pi <- c(rep(b1, q), rep(0, p - q))
26
27   d <- X %*% pi + rnorm(n)
28   y <- theta * d + X %*% beta + rnorm(n)
29
30   df <- data.frame(cbind(y, d, X))
31   colnames(df)[1:2] <- c("y", "d")
32
33   dml <- rlassoEffect(x = X, y = y, d = d, method = "double selection")
34   post.lasso <- rlasso(y ~ d + ., post=T, intercept=F, data=df)
35
36   res[i, "dml1"] <- coef(dml)["d1"]
37   res[i, "post.lasso1"] <- coef(post.lasso)["d"]
38 }
39
40 #####
41 ### 2. M-graph
42 #####
43 for (i in 1:s){
44   u1 <- rnorm(n)
45   u2 <- rnorm(n)
46
47   # bad controls
48   x1 <- matrix(rnorm(n * q), ncol = q) + sqrt(b1) * u1 + sqrt(b2) * u2
49   # irrelevant controls
50   x2 <- matrix(rnorm(n * (p - q)), ncol = (p - q))
51   X <- cbind(x1, x2)
52   colnames(X) <- paste("X", 1:p, sep = " ")
53
54   d <- sqrt(b1) * u1 + rnorm(n)
55   y <- theta * d + sqrt(b2) * u2 + rnorm(n)
56
57   df <- data.frame(cbind(y, d, X))
58   colnames(df)[1:2] <- c("y", "d")
59
60   dml <- rlassoEffect(x = X, y = y, d = d, method = "double selection")
61   post.lasso <- rlasso(y ~ d + ., post=T, intercept=F, data=df)

```

```

62
63   res[i, "dml2"] <- coef(dml)[ "d1" ]
64   res[i, "post.lasso2"] <- coef(post.lasso)[ "d" ]
65 }
66
67 #####
68 ### 3. Mediator
69 #####
70 for (i in 1:s){
71   d <- rnorm(n)
72
73   x1 <- matrix(rnorm(n * q), ncol = q) + b1 * d
74   x2 <- matrix(rnorm(n * (p - q)), ncol = (p - q))
75   X <- cbind(x1, x2)
76   colnames(X) <- paste("X", 1:p, sep = " ")
77
78   beta <- c(rep(b2, q), rep(0, p - q))
79   y <- theta * d + X %*% beta + rnorm(n)
80
81   df <- data.frame(cbind(y, d, X))
82   colnames(df)[1:2] <- c("y", "d")
83
84   dml <- rlassoEffect(x = X, y = y, d = d, method = "double selection")
85   post.lasso <- rlasso(y ~ d + ., post=T, intercept=F, data=df)
86
87   res[i, "dml3"] <- coef(dml)[ "d1" ]
88   res[i, "post.lasso3"] <- coef(post.lasso)[ "d" ]
89 }
90
91 #####
92 ### 4. Confounded Mediator
93 #####
94 for (i in 1:s){
95   d <- rnorm(n)
96   u <- rnorm(n)
97
98   x1 <- matrix(rnorm(n * q), ncol = q) + b1 * d + sqrt(b2) * u
99   x2 <- matrix(rnorm(n * (p - q)), ncol = (p - q))
100   X <- cbind(x1, x2)
101   colnames(X) <- paste("X", 1:p, sep = " ")
102
103   beta <- c(rep(b2, q), rep(0, p - q))
104   y <- theta * d + X %*% beta + sqrt(b2) * u + rnorm(n)
105
106   df <- data.frame(cbind(y, d, X))
107   colnames(df)[1:2] <- c("y", "d")
108
109   dml <- rlassoEffect(x = X, y = y, d = d, method = "double selection")
110   post.lasso <- rlasso(y ~ d + ., post=T, intercept=F, data=df)
111
112   res[i, "dml4"] <- coef(dml)[ "d1" ]
113   res[i, "post.lasso4"] <- coef(post.lasso)[ "d" ]
114 }

```
